# Supplementary material for: Minimum-Risk Recalibration of Classifiers
Source: arXiv:2305.10886 source file (2023-05-18)
Supplement: Supplementary file 3 [file appendixB_proof_calibration.tex]

\section{Proof of Theorem \ref{Thm:risk_bound}}\label{sec:proof_risk_recalib}

\DS{TODO: Add a preamble that outlines the proof strategy here.}

We first define two events for for some $B \in \NN$ and $D > 0$:
\begin{align}
    \textrm{2-well-balanced binning:} \quad &E_1(B) = \left\{\frac{1}{2 B} \leq \bbP[Z\in I_b] \leq \frac{2}{B},   \quad \forall b \in [B].\right\}, \label{eq:E1} \\
    \textrm{Accurate bin average estimation:} \quad &E_2(D) = \{|\hat{\mu}_b - \mu_b| \leq D, \quad \forall b\in [B]\}. \label{eq:E2}
\end{align}
Under $E_1(B)$, the uniform-mass binning scheme of size $B$ is 2-well balanced. Under $E_2(D)$, the average in each bin concentrates within $D$ to the conditional expectation uniformly for all bins.

\todo{introduce lemmas and proof sketch}
Theorem~\ref{Thm:risk_bound} provides a high probability bound on the risk of the recalibration function $\hh = \sum_{b=1}^B \hat{\mu}_b \cdot \indic_{I_b}(z)$. According to Proposition \ref{Prop:risk_decomposition}, the risk of $\hh$ can be decomposed into two components:
\begin{align}
    R(\hh; f, P) = \REL\left( \hh \circ f; P \right) + \GRP \left( \hh; f, P \right).
\end{align}
We can bound the risk with high probability by providing bounds on $\REL$ and $\GRP$ under certain high probability events.

% Lemma~\ref{LEMMA:WELL} states that $E_1$

% The recalibration function $\hh = \sum_{b=1}^B \hat{\mu}_b \cdot \indic_{I_b}(z)$ is constructed in two steps: (1) binning: estimating $I_b$'s using quantiles, and (2) estimating: estimating $\mu_b$ in each bin. Define two events. Under the first event $E_1$, the binning is accurately enough; under the second event $E_2$, the estimating is accurately enough.
% under which the binning

\subsection{Well-balanced Binning}
Recall the notion of well-balanced binning from Definition \ref{defn:binning_balanced}: for any $B \in \NN$ and any $\alpha \geq 1$, a binning scheme $\cB = \left\{ I_1, \dots, I_B \right\}$ of size $B$ is $\alpha$-well balanced if
\[
    \frac{1}{\alpha B} \leq \bbP[Z\in I_b] \leq \frac{\alpha}{B}, \quad \forall b \in [B].
\]
The following lemma shows the uniform-bass binning scheme $\mathcal{B}$ is 2-well-balanced with high probability for sufficiently large sample size. 

% \DS{Is this lemma (along with its proof) the same with what's presented in the original reference, or is it any different?  If they are the same, why do we copy the proof here?}

% \todo{Generalize to arbitrary $\alpha$}
\begin{lemma}[{\cite[][Lemma 4.3]{kumar2019verified}}]
\label{LEMMA:WELL}
There exists a universal constant $c$ such that for any $\delta \in (0,1)$, if $n \geq cB \log (B/\delta)$, with probability at least $1 - \delta$, the event $E_1(B)$ holds.
That is,
$$
P[\textrm{the uniform-mass binning scheme $\mathcal{B}$ is 2-well-balanced}] \geq 1 - \delta.
$$
\end{lemma}

\DS{Following their proof, we may choose $c = 2420$}

\subsection{Accurate bin average estimation}

% Before we consider the reliability loss, we first need the following lemma that controls the estimation error of bin values uniformly for all bins. 
\begin{lemma}[Uniform reliability error control {\cite[][Corollary 1]{gupta2021withoutsplitting}}]
\label{LEMMA:FREE}
    Assume $P_Z$ is absolutely continuous and $n \geq 2B$. Under the uniform-binning scheme $\mathcal{B}$ with size $B$, for any $\delta \in (0,1)$, the event $E_2\left( D \right)$ holds with probability at least $1-\delta$, where
    $$D = \sqrt{\frac{\log (2B/\delta)}{2(n/B - 1)}} + \frac{B}{n}.$$
    That is,
    $$P\left[ |\hat{\mu}_b - \mu_b| \leq \sqrt{\frac{\log (2B/\delta)}{2(n/B - 1)}} + \frac{B}{n} \quad \forall b\in[B]\right] \geq 1-\delta.$$
\end{lemma}

\subsection{Reliability Risk}
% Next, under the event $E_1$ and $E_2$ specified in Equation~(\ref{eq:E1}) and (\ref{eq:E2}), we consider the bound for reliability loss.

% Assuming the same conditions as Lemma~\ref{LEMMA:WELL} but with a larger sample size of $n=\Omega(B^2\log B)$, we obtain $\REL = O(1/\sqrt{B})$ as $B\to \infty$. This result is formally presented in the following lemma.

\begin{lemma}[Reliability loss bound]
\label{Lemma:REL}
    Under the event $E_1(B)$ and $E_2(D)$,
    $$\REL(\hat{h} \circ f; P) \leq \alpha D.$$
\end{lemma}

\begin{proof}[Proof of Lemma \ref{Lemma:REL}]
\begin{align}
    \REL(\hat{h} \circ f; P) &= E[(\hat{h}(Z) - E[Y|\hat{h}(Z)])^2] \\
    &\leq E[|\hat{h}(Z) - E[Y|\hat{h}(Z)]|] \label{eq:60} &(Y\in\{0,1\}) \\
    &= \sum_{b=1}^B P[\hat{\beta}(Z)=b] |\hat{\mu}_b - \mu_b| \\
    &\leq \sum_{b=1}^B \frac{\alpha}{B} |\hat{\mu}_b - \mu_b|
    &\qquad \textrm{(under $E_1(B)$)} \\
    &\leq \sum_{b=1}^B \frac{\alpha}{B} D
    &\qquad \textrm{(under $E_2(D)$)} \\
    &= \alpha D
\end{align}
\end{proof}

% \begin{remark}
% Under the assumptions of Theorem~\ref{Thm:REL} but with a larger sample size $n=cB^2\log(4B/\delta)$, with probability at least $1-\delta$, we have
% \begin{align}
%     \REL(\hat{h}(Z))
%     &\leq \sqrt{\frac{2B}{n}\log\frac{4B}{\delta}} \leq \sqrt{\frac{2}{cB}} = O(B^{-1/2}) \quad \textrm{ as $B\to\infty$}.
% \end{align}
% \end{remark}

\subsection{Grouping Risk}

\begin{lemma}[Grouping loss bound]\footnote{\zs{Similar to the combination of Lemma D.5 and D.6 in {\cite{kumar2019verified}}. Differences are: (1) we have better constant 1 as opposed to 2 in {\cite[][Lemma D.5]{kumar2019verified}}, and (2) we use $Z$ as opposed to $g(Z)$ in {\cite{kumar2019verified}}.}}
\label{Lemma:GRP}
    If $h^*$ is monotonically non-decreasing, then,
    under the event $E_1(B)$,
    $$\GRP(\hat{h}; f, P) \leq \frac{\alpha}{B}$$
\end{lemma}

\begin{proof}[Proof of Lemma \ref{Lemma:GRP}]
Define $\beta:[0,1]\to [B]$ as $\beta(z) = b$ if $z \in I_b$; that is, $\beta(z)$ gives the index of the unique bin that contains $z$.
\begin{align}
    \GRP(\hat{h}; f, P) &= E[(E[Y|\hat{h}(Z)] - E[Y|Z])^2] \\
    &\leq E[|E[Y|\hat{h}(Z)] - E[Y|Z]|] &(Y\in\{0,1\}) \\
    &= E[E[|E[Y|\hat{h}(Z)] - E[Y|Z]| | \hat{\beta}(Z)]] &\textrm{(towering property)} \\
    &\leq E\left[\mu_{\hat{\beta}(Z)} - \mu_{\hat{\beta}(Z) - 1}\right] &\textrm{($h^*$ is monotonically increasing)} \\
    &= \sum_{b=1}^B P[\hat{\beta}(Z) = b] (\hat{\mu}_{b} - \hat{\mu}_{b - 1}) \\
    &\leq \sum_{b=1}^B \frac{\alpha}{B} (\mu_{b} - \mu_{b - 1}) &\textrm{(under $E_1(B)$)}\\
    &\leq \frac{\alpha}{B}.
\end{align}
\end{proof}

\subsection{Completing the Proof of Theorem \ref{Thm:risk_bound}}
\riskbound*
\begin{proof}[Proof of Theorem~\ref{Thm:risk_bound}]
    For any $\delta \in (0,1)$, by Lemma~\ref{LEMMA:WELL}, there is a constant $c_1 > 0$ such that
    \begin{align}
        P[E_1(B)] \geq 1 - \delta,
    \end{align}
    if $n \geq c_1 B \log(B/\delta)$.
    Additionally, if we require $n \geq c B\log(B/\delta)$ where $c = \max \{c_1, 2/\log(B/\delta)\}$, then we have $n \geq 2B$. Since $n \geq 2B$ and $P_Z$ is absolutely continuous, by Lemma~\ref{LEMMA:FREE}, we have 
    \begin{align}
        P[E_2(D)] \geq 1 - \delta,
    \end{align}
    where $D = \sqrt{\frac{\log (2B/\delta)}{2(n/B - 1)}} + \frac{B}{n}$.
    Applying union bound, we have
    \begin{align}
        P[E_1(B) \cap E_2(D)] \geq 1 - 2 \delta \label{eq:E1_2}
    \end{align}
    if $n \geq c B\log(B/\delta)$.
    
    Under $E_1(B)$ and $E_2(D)$, since $h^*$ is monotonically non-decreasing, we have, by Lemma~\ref{Lemma:REL} and \ref{Lemma:GRP},
    \begin{align}
        \REL(\hat{h}\circ f; P) &\leq 2 D, \label{eq:REL_bound} \\
        \GRP(\hat{h}; f, P) &\leq \frac{2}{B}, \label{eq:GRP_bound}
    \end{align}
    and, as a consequence of Proposition~\ref{Prop:risk_decomposition},
    \begin{align}
        R(\hat{h}) &= \REL(\hat{h}\circ f; P) + \GRP(\hat{h}; f, P) \notag \\
        &\leq 2\left(D + \frac{1}{B}\right). \label{eq:R_bound}
    \end{align}   
    
    Considering Equation~(\ref{eq:E1_2}), we conclude the bounds in Equation~(\ref{eq:REL_bound})-(\ref{eq:R_bound}) holds with probability at least $1-2\delta$ if $n \geq c B\log(B/\delta)$.
\end{proof}
